# Supplementary material for: Class-Level Code Generation from Natural Language Using Iterative, Tool-Enhanced Reasoning over Repository
Source: arXiv:2405.01573 source file (2024-06-05)
Supplement: Supplementary file 1 [file language_specific.tex]

\section{Language specific details}

\subsection{\Java}

\begin{itemize}
    \item The Java dataset is constructed using existing data gathered by MGD.
    
    \item Step 1: Gather classes with repository dependencies.
    \begin{itemize}[label=$\circ$]
        \item Identify classes that have at least one dependency on the repository.
        \item Dependencies include classes, methods, or variables used in various ways such as inheritance, method parameters, or utility functions.
    \end{itemize}
    
    \item Step 2: Validate corresponding test cases for each class.
    \begin{itemize}[label=$\circ$]
        \item Ensure each class has corresponding test cases.
        \item Validate test cases by checking if the class is referenced in the test code.
        \item Ensure at least 2/3rds of the class methods are covered by the tests.
    \end{itemize}
    
    \item Step 3: Verify test cases pass on ground truth.
    \begin{itemize}[label=$\circ$]
        \item Delete the class from the repository to check if tests fail.
        \item Re-introduce the class to ensure tests pass without failure.
        \item Ensures tests fail when the correct class implementation is absent and pass with the correct implementation.
    \end{itemize}
    
    \item Step 4: Generate metadata including class and method details.
    \begin{itemize}[label=$\circ$]
        \item Generate structured metadata for each class.
        \item Metadata includes class name, access specifier, parent class (if applicable), variables, method signatures, and docstrings.
        \item Docstrings are generated using GPT-4 if not provided in the ground truth.
    \end{itemize}
    
    \item Step 5: Create natural language descriptions using metadata.
    \begin{itemize}[label=$\circ$]
        \item Generate two types of descriptions for each class.
        \begin{itemize}[label=\textendash]
            \item Detailed description retaining all metadata information.
            \item Brief description removing method definitions but retaining other details.
        \end{itemize}
        \item Descriptions created using GPT-4.
    \end{itemize}
    
\end{itemize}

\subsection{\Python}

\subsection{\CSharp}
