# Supplementary material for: Class-Level Code Generation from Natural Language Using Iterative, Tool-Enhanced Reasoning over Repository
Source: arXiv:2405.01573 source file (2024-06-05)
Supplement: Supplementary file 2 [file related_works.tex]

\section{Related Works}
\subsection{Papers on Language Models with Reasoning, Acting, and Tool Integration}

\begin{itemize}
\item \textbf{ReAct: Synergizing Reasoning and Acting in Language Models} \cite{tools:react}: This paper introduces the ReAct framework, which explores the use of large language models to generate both reasoning traces and task-specific actions in an interleaved manner, enhancing synergy between reasoning and acting components.

\item \textbf{Toolformer: Language Models Can Teach Themselves to Use Tools} \cite{tools:toolformer}: Toolformer demonstrates that language models can teach themselves to use external tools via simple APIs improving zero-shot performance across various downstream tasks.

\item \textbf{Augmented Language Models: a Survey} \cite{tools:toolssurvey}: This survey paper reviews works in which language models are augmented with reasoning skills and the ability to use external tools. It discusses the potential of augmented language models (ALMs) to address limitations of traditional language models.

\item \textbf{FireAct: Toward Language Agent Fine-tuning} \cite{tools:fireact}: This paper investigates the fine-tuning of language models on ReACT trajectories to enhance language agents' performance across tool-related tasks.

\item \textbf{ToolkenGPT: Augmenting Frozen Language Models with Massive Tools via Tool Embeddings} \cite{tools:toolken}: ToolkenGPT offers a novel approach to augment language models with external tools using tool embeddings, improving tool use in various domains.

\item \textbf{GEAR: Augmenting Language Models with Generalizable and Efficient Tool Resolution} \cite{tools:gear}: GEAR introduces a computationally efficient query-tool grounding algorithm that is scalable to large tool libraries and novel tasks.

\end{itemize}

\subsection{Papers on Code Generation using Tool Integration}

\begin{itemize}
\item \textbf{ToolCoder: Teach Code Generation Models to use API search tools} \cite{}: ToolCoder proposes an approach to integrate API search tools with code generation models to assist in code generation and API selection, demonstrating improved performance on code generation benchmarks.
\item \textbf{Copiloting the Copilots: Fusing Large Language Models with Completion Engines for Automated Program Repair
} \cite{lsp:copiloting_copilots_uiuc}
\end{itemize}

\subsection{Papers on Context Understanding in Code Completions}

\begin{itemize}
\item \textbf{RepoFusion: Training Code Models to Understand Your Repository} \cite{cr:repofusion}: RepoFusion focuses on training models to incorporate relevant repository context, demonstrating improved code completion performance in scenarios where context understanding is crucial.

\item \textbf{Repo-Level Prompt Generator: Enhancing Large Language Models for Code Assistance} \cite{cr:rlpg}: Repo-Level Prompt Generator introduces a framework for enhancing code completion using large language models (LLMs) like Codex. It generates example-specific prompts based on context from the entire code repository, improving code autocompletion performance. This approach doesn't require access to LLM weights, making it versatile. 

\item \textbf{RepoCoder: Streamlining Repository-Level Code Completion} \cite{cr:repocoder}: RepoCoder offers a solution for repository-level code completion, addressing the challenge of utilizing scattered information across files. It combines a similarity-based retriever and a pre-trained code language model to effectively leverage repository-level context for code completion. RepoCoder employs an iterative retrieval-generation approach and introduces RepoEval, a new benchmark. 

\end{itemize}

\subsection{Benchmark papers}
\begin{itemize}
\item \textbf{ClassEval: A Manually-Crafted Benchmark for Evaluating LLMs on Class-level Code Generation} \cite{bench:classeval}: This paper evaluates language models on class-level code generation tasks, highlighting differences in performance compared to method-level code generation benchmarks.
\item Cross-code eval
\end{itemize}
